# Supplementary material for: Exploiting Student Parallelism for Efficient GPU Inference of BERT-like Models in Online Services
Source: arXiv:2408.12526 source file (2025-03-18)
Supplement: Supplementary file 1 [file exp_appendix.tex]

\section{Additional Experiment Results}
\begin{figure}[t]
	
	\includegraphics[width=\linewidth]{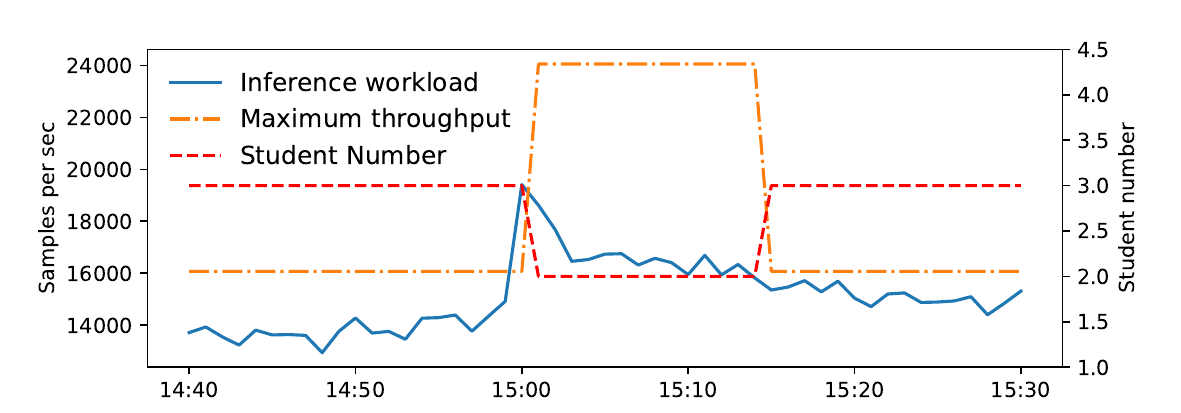}
	\caption{How student number adapted to the dynamic workloads for better throughput}
	\label{fig:adaptiv_student_case}
 \vspace{-5mm}
\end{figure}
\subsection{Case Study in Adaptive Student Number} 
We also make a case study on how the student number adapted to dynamic workloads for better throughput on 4 GPUs. 
%We use the MRPC dataset from an online search engine, which scores the relevance of hundreds of filtered documents for each query. 
We extract a period of workload trace that have workload burst to run this experiment.
As shown in Figure~\ref{fig:adaptiv_student_case}, the student number is three at first, namely the best-pruned number. 
When there is a workload peak, it reduces the student number to two for better throughput to empty the length-aware buffer.
Until the workload is lower and enough workers are idle for the time threshold, it improves the student number to three again for better prediction quality.

\subsection{Scalability}

\begin{figure}[t]
	\includegraphics[width=0.95 \linewidth]{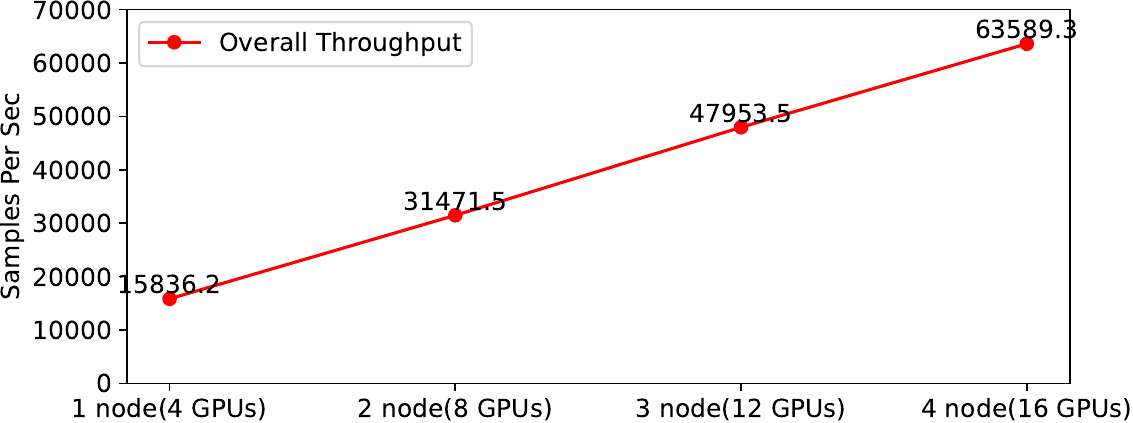}
	\caption{The scalability: overall throughput increases almost linearly with the node and GPU number}
	\label{fig:scalability}
\end{figure}

As shown in Figure~\ref{fig:scalability}, our \sys has the good scalability, 
since the overall inference throughput increases almost linearly with the number of nodes and GPUs.
Every node has its own student groups, length-aware buffer, and resource management.
With more nodes added, not only the inference execution but also the logical controller have more resources to scale up for more inference samples.
The global dispatcher has high throughput, because it schedules workloads in the simple round-robin method.
